# Supplementary material for: Interfering tunneling paths through magnetic molecules on superconductors: Asymmetries of Kondo and Yu-Shiba-Rusinov resonances
Source: arXiv:2007.12092 source file (2020-07-23)
Supplement: Supplementary file 1 [file SM_Fig1.pdf]

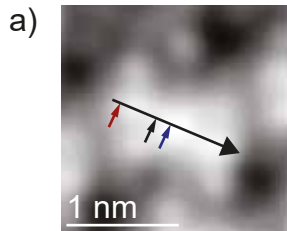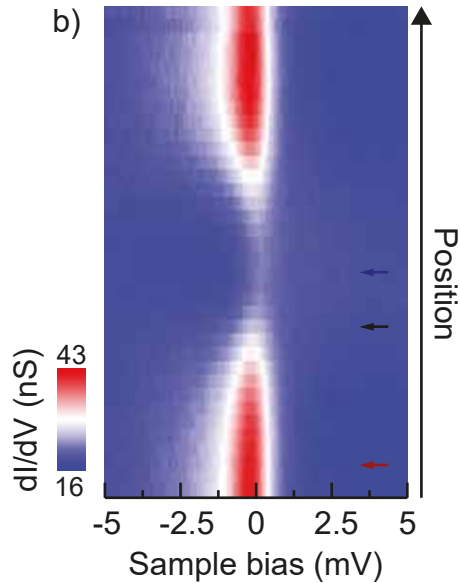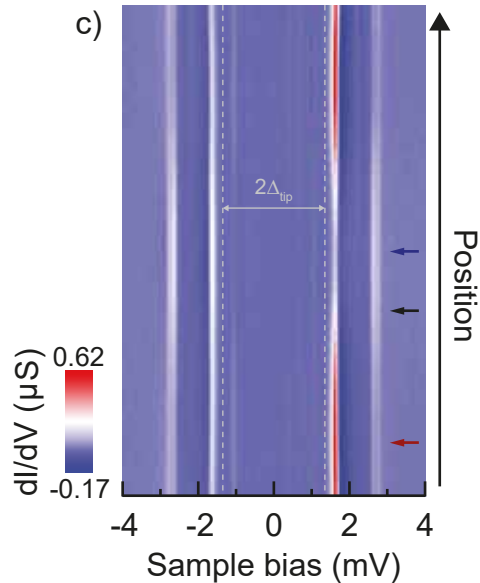

# Sampling bias in
